# Supplementary material for: Robobarista: Object Part based Transfer of Manipulation Trajectories from Crowd-sourcing in 3D Pointclouds
Source: arXiv:1504.03071 source file (2015-09-18)
Supplement: Supplementary file 1 [file appendix.tex]

%\section*{Appendix}

\begin{figure*}[tb]
\begin{center}
\includegraphics[width=0.90\textwidth]{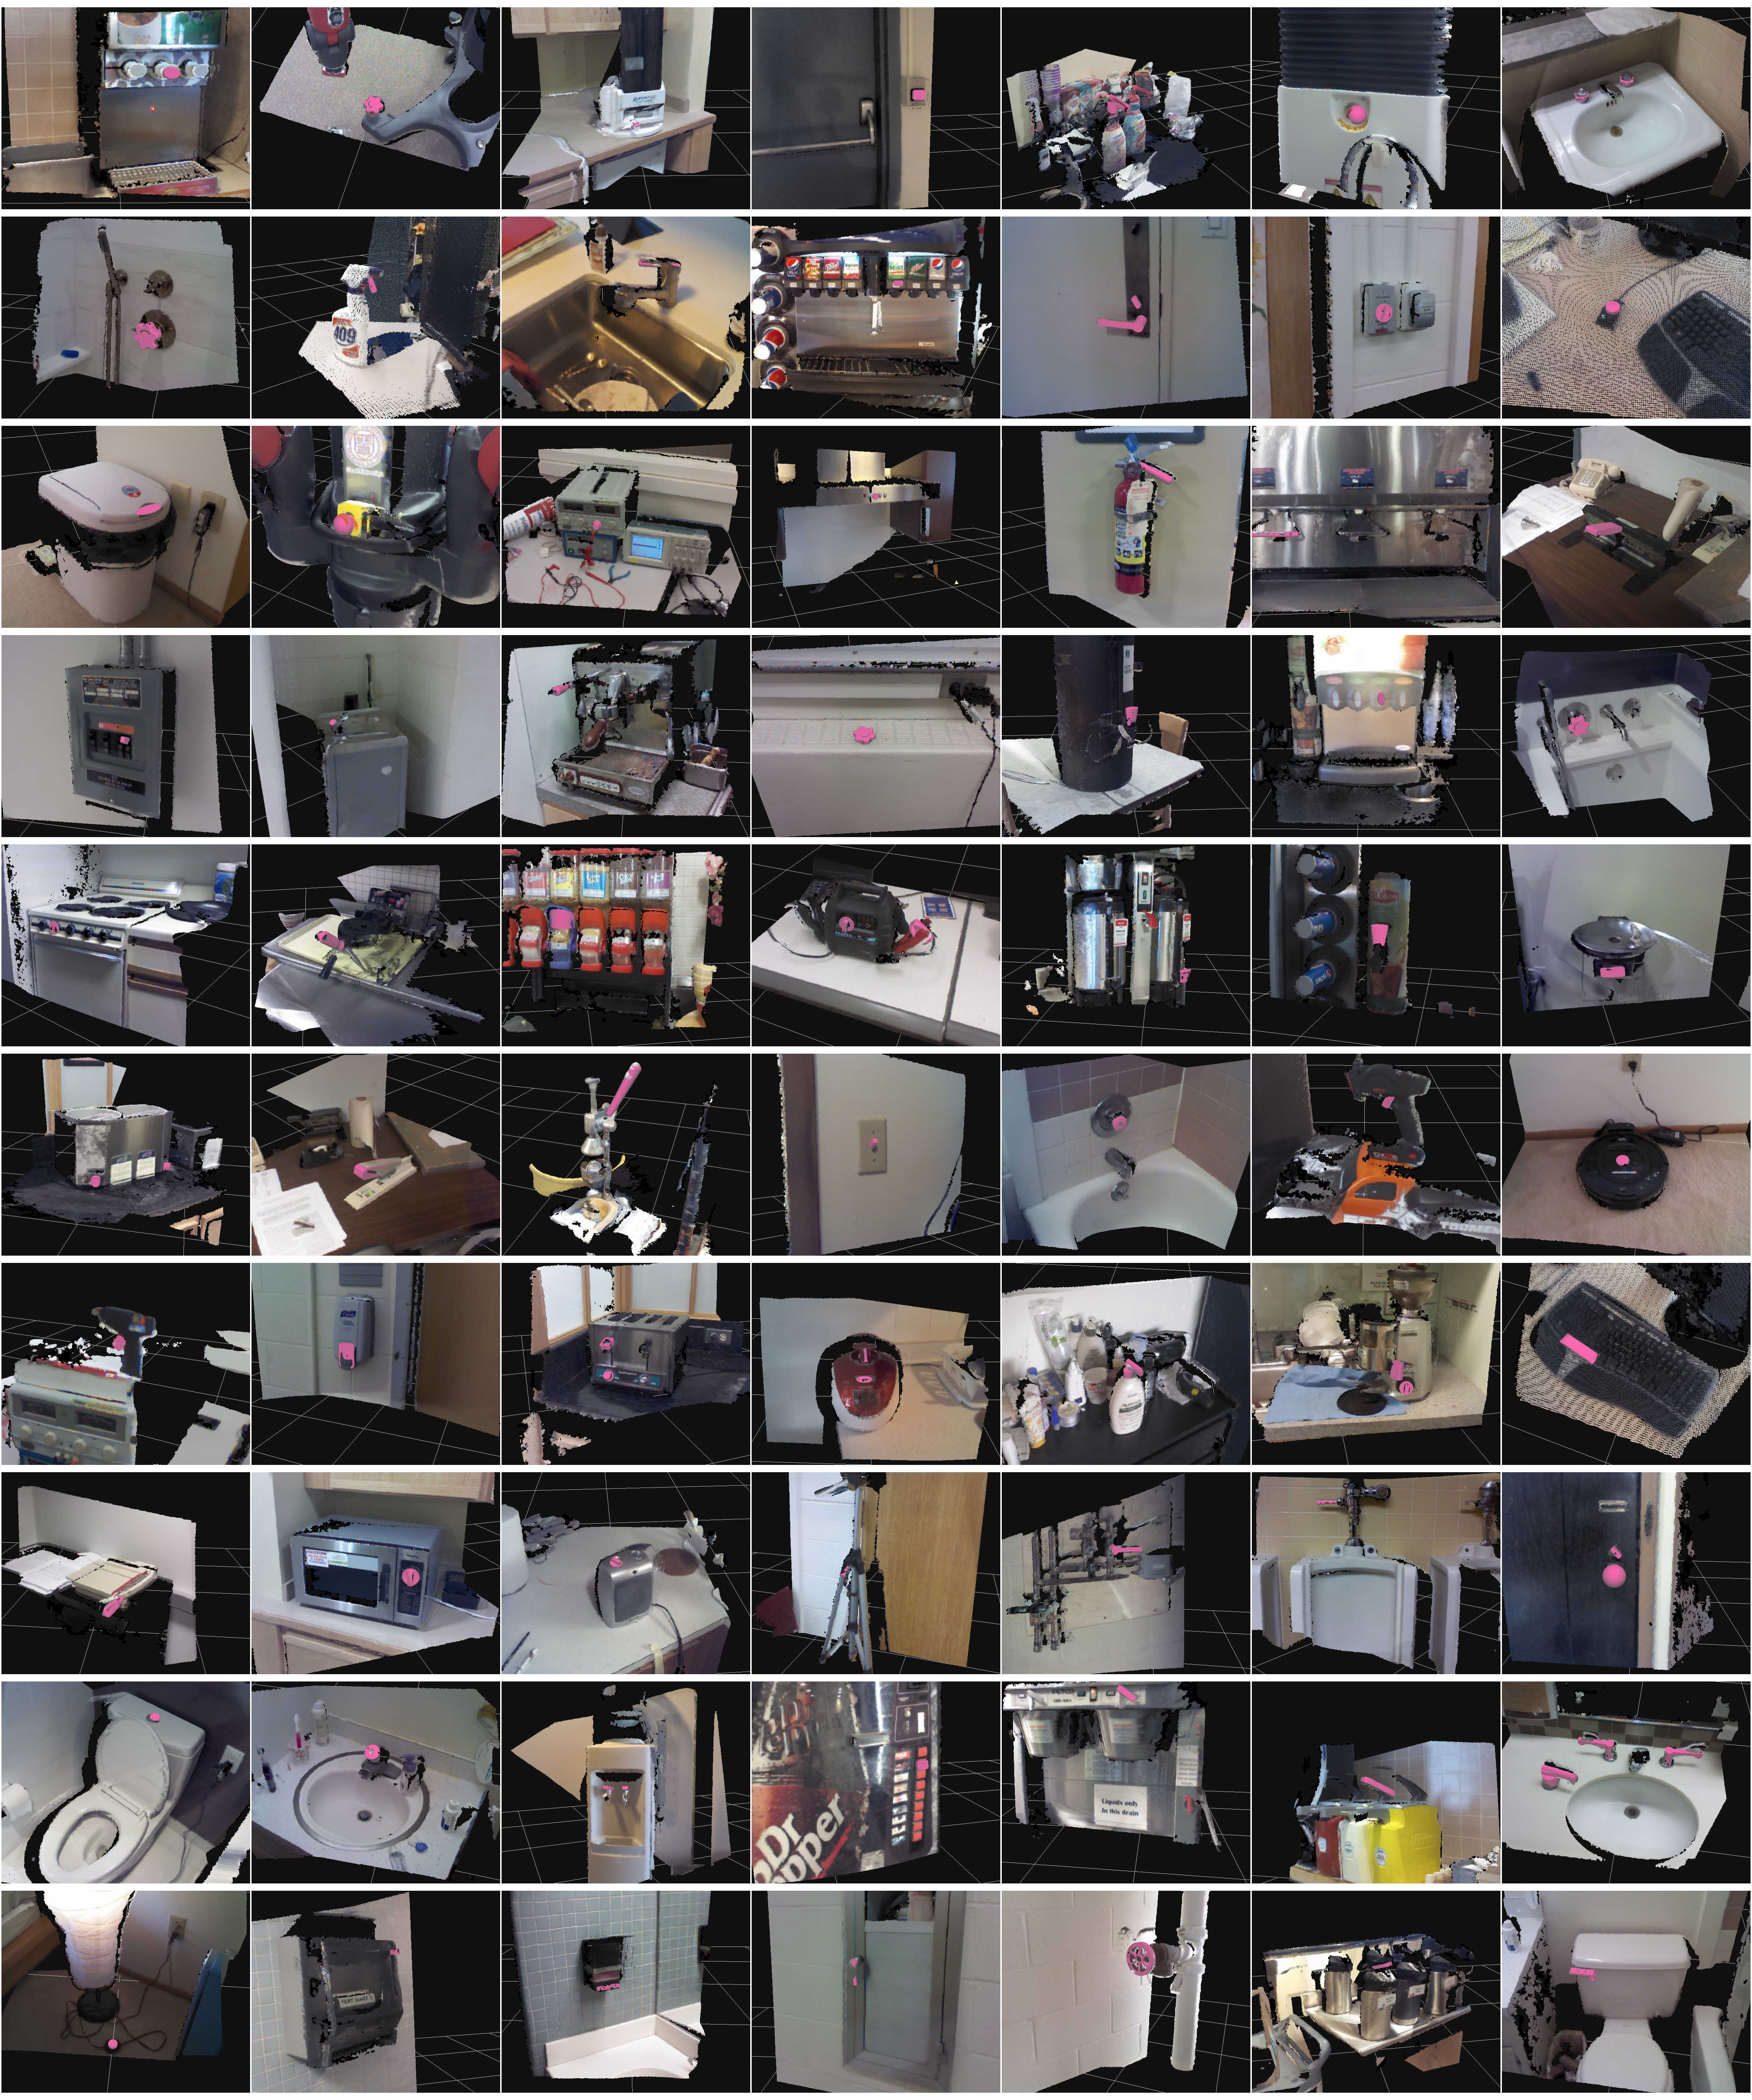}
\end{center}
\caption{
\textbf{Examples of objects and object parts} 
from our dataset of 116 objects and 249 parts.
Each image shows the point cloud
representation of an object and one of its parts highlighted.
%, with one of its object part overlaid by CAD model highlighted.
}
\label{fig:all_objects}
\end{figure*}
